# Supplementary material for: Atomic-scale relaxation dynamics and aging in a metallic glass probed by X-ray photon correlation spectroscopy
Source: arXiv:1209.2030 source file (2012-09-10)
Supplement: Supplementary file 1 [file SupplementalMaterial.pdf]

# Supplementary information

## Materials

The $Mg_{65}Cu_{25}Y_{10}$ metallic glass was obtained by prealloying Cu-Y ingots with the adequate ratio in an arc-melter furnace under a Ti-gettered argon atmosphere and then alloying with magnesium in an induction furnace. The melt (~1250 K) was fast-quenched with a cooling rate of $10^6$ K/s by injecting it on a copper spinning wheel in a melt spinner device. The resulting ribbons had a thickness of ~33 μm and a width of ~2 mm. The amorphous structure of the samples was checked by high resolution X-ray diffraction.

## XPCS thermal protocols:

XPCS data were acquired during isothermal steps of at least one hour each. In all experiments a fixed heating/cooling rate of 1 K/min has been used for temperature changes in between the constant T steps.

**AQ-g:** Glass obtained by quenching the corresponding melt to T = 300 K at a very fast cooling rate of $10^6$ K/s. This glass has been measured with XPCS by performing several isothermal steps, starting from 300 K up to 408 K.

**Supercooled liquid and SC-g**: Supercooled liquid obtained after increasing further the temperature of the AQ-g above T=408 K and glass obtained by the subsequent cooling of the melt below $T_g$, down to 373 K, always using a rate of 1 K/min. Differently from the AQ-g, the data in the SC-g are taken on lowering the temperature.

**AQ-g2:** As-quenched glass, produced by quenching the corresponding melt to T = 300 K at a very fast cooling rate of $10^6$ K/s and then slowly heating the glass at 1 K/min up to T= 415 K for a first measurement, before lowering the temperature down to 403 K at 1 K/min for a second run.

## Differential Scanning Calorimetry (DSC)

The glass transition temperature was measured by means of a Perkin Elmer DSC-7 with a resolution below 1 μW. Several as-quenched glasses were heated at 5, 10 and 20 K/min up to the supercooled liquid phase and then cooled again down to room temperature, and the specific heat measurements were carried out also on the corresponding slowly cooled glasses (SC-g). The heating and cooling rates were equivalent. A baseline was estimated using a completely crystallized sample. The value of $T_g$ at 1 K/min for the SC-g was estimated from the analysis of the heating rate dependence of the measured glass transition temperatures, as shown in the Supplementary Information. Values for the structural relaxation time for SC-g are obtained by using the relation $\tau(R)=\Delta T_g/R$ for the different $T_g(R)$, being $\Delta T_g$ the temperature interval corresponding to the glass transition and R the heating rate [1].

Figure S1 reports the endothermic heat flow measured with DSC in both an AQ-g glass and in the SC-g glass obtained after temperature cycling above and below $T_g$ with a fixed heating/cooling rate of 5 K/min.

AQ-g displays a minimum in the glassy state which is not present in SC-g, followed by a lower peak at temperatures higher than $T_g$. These features are the typical consequence of the annealing produced by the very slow heating rate with respect to the cooling rate used to produce the glass. They correspond indeed to a loss of enthalpy in the glassy state, which is then recovered in the SC-g glass.

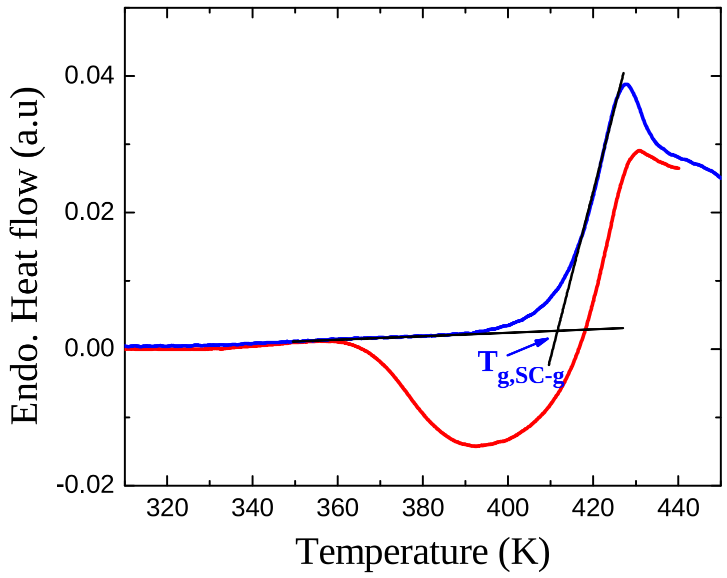


**Figure S1:** DSC profile measured for both AQ-g (blue line) and SC-g (red line) at a fixed heating/cooling rate of 5 K/min.

As shown in Figure S1, the intersection of two lines fitting the increasing heat flow above $T_g$ and the value in the glassy state allows determining the calorimetric glass transition temperature for the SC-g. The dependence of $T_g$ on the heating rate can be used to estimate the value of $T_g$ at the rate R=1 K/min used in the XPCS experiments [2]. Figure S2 shows the logarithm of the heating rate as function of the inverse of the calorimetric glass transition. From the observed linear behaviour we find $T_g$= 405 K for R=1 K/min.

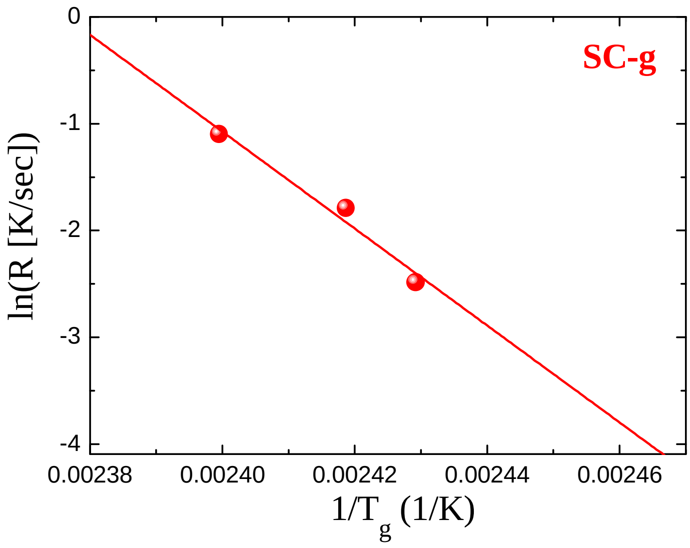


**Figure S2:** Heating rate dependence of the calorimetric glass transition temperature for the SC-g.

## Dynamic Mechanical Analyzer (DMA)

Mechanical spectroscopy was realized with a TA instrument Q800 Dynamic Mechanical Analyzer. The experiments were realized in tension mode by fixing ribbon pieces ~10 mm long with a preload force of 0.08 N. The amplitude of the oscillation was fixed to ~1 µm. Both preload and amplitude values were found to be adequate in order to avoid the failure of the ribbons during the softening associated to the glass transition. Data were collected with a constant heating rate of 1 K/min by using different frequency values ranging from 0.1 to 100 Hz. The maximum temperature of the heating ramps (~445 K) was determined by the decrease in viscosity, provoking the material to flow easily under the preload stress. No sign of stiffening due to crystallization was observed. Structural relaxation times have been directly obtained from the position of the peak in the imaginary part of the elastic modulus in the liquid phase.

Figure S3 shows the temperature evolution of the Young modulus measured by DMA at a frequency of 1 Hz, in both the AQ-g and SC-g. The storage modulus of the AQ-g (orange line) displays a very low value with respect to the one corresponding to SC-g (red line), up to 360 K, where it significantly increases in a narrow temperature range. This raise is due to release of free volume and internal stresses upon heating the system with a lower rate with respect to the rate used to prepare the glass. Variations in both density and shape of the ribbons contribute as well to the huge change displayed in the Figure between the two glassy states.

By contrast, the storage modulus of the SC-g (red line) glass exhibits an almost constant value up to the onset of the dynamic glass transition. The corresponding loss modulus (cyan line) shows instead the typical loss peak at 440 K, in the liquid phase. This temperature corresponds to a characteristic structural relaxation time $\tau=1/2\pi f$, where f is the applied frequency.

In the glassy state, the AQ-g glass (blue line) displays a small excess in the loss modulus between 360 K and 410 K, which is related to the release of internal stresses associated to the slow heating rate.

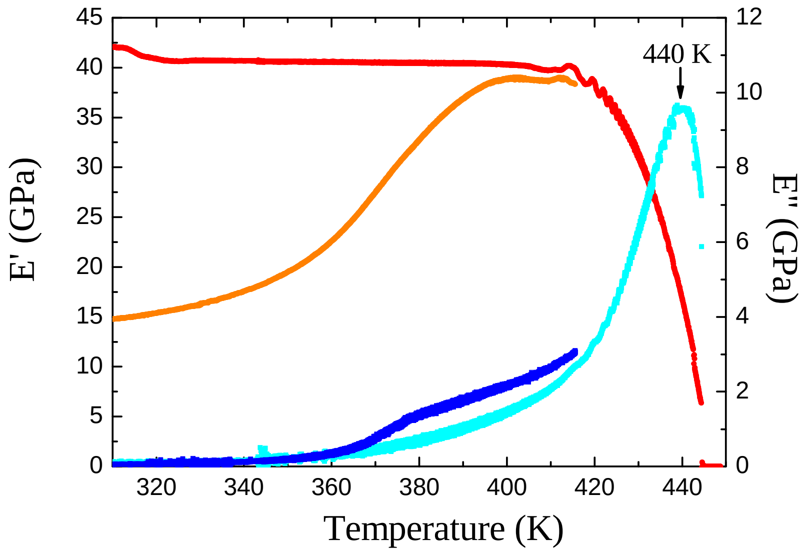


**Figure S3:** Temperature evolution of the real (red and orange symbols, left y-axis) and imaginary part (blue and cyan symbols, right y-axis) of the Young modulus measured by DMA . The data are collected using a constant heating rate of 1 K/min and a frequency of 1 Hz, for both the AQ-g (orange and blue curves) and the SC-g (red and cyan curves).

## Aging and equilibrium dynamics in the SC-g and in the supercooled liquid

Figure S4 shows the temperature dependence of the structural relaxation time (a) and the shape parameter β (b) measured with XPCS in the SC-g glass and in the supercooled liquid. In the glassy state the system is in the intermediate aging regime where both τ and β depend on waiting time (arrows) and the time-waiting time-temperature superposition principle does not hold.

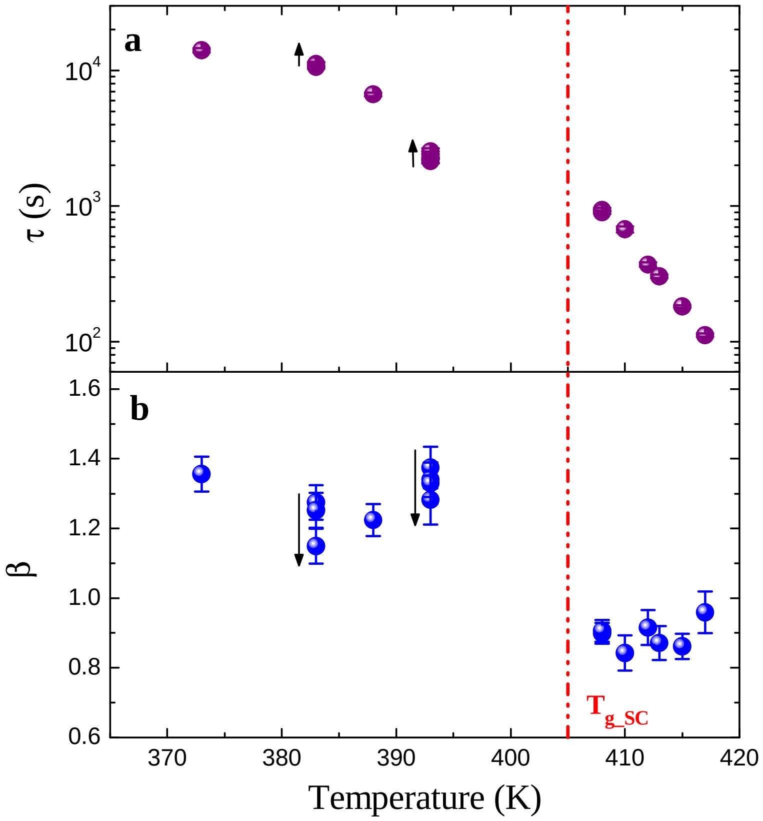


**Figure S4. a,** Temperature dependence of the structural relaxation time in the SC-g (below 405 K) and supercooled liquid (above 405 K), measured with XPCS. **b,** Corresponding shape parameter β as a function of temperature. In both panels the arrows indicate the evolution with the sample age and the dashed red line marks the calorimetric glass transition temperature of the SC-g.

## REFERENCES

1. R. Busch, R. Bakke, and W. L. Johnson, Acta Mater. **46**, 4725 (1998).
2. C. T. Moynihan, A. J. Easteal, and J. Wilder, J. Phys. Chem. **78,** 2673-2677 (1974).
